# Supplementary material for: Full multipartite steering inseparability, genuine multipartite steering and monogamy for continuous variable systems
Source: arXiv:2108.06926 source file (2021-12-31)
Supplement: Supplementary file 1 [file supp_material.pdf]

# Supplemental Materials

Run Yan Teh[1], Manuel Gessner[2,3], Margaret D. Reid[1] and Matteo Fadel[4]
[1]*Centre for Quantum Science and Technology Theory,*
*Swinburne University of Technology, Melbourne, Australia*
[2]*Laboratoire Kastler Brossel, ENS-Université PSL, CNRS, Sorbonne Université,*
*College de France, 24 Rue Lhomond, 75005, Paris, France*
[3]*ICFO-Institut de Ciències Fotòniques, The Barcelona Institute of Science and Technology,*
*Av. Carl Friedrich Gauss 3, 08860, Castelldefels (Barcelona), Spain and*
[4]*Department of Physics, University of Basel,*
*Klingelbergstrasse 82, 4056 Basel, Switzerland*

## I. COMPARISON WITH RESULTS OF WANG ET AL.

In this section, we show the correlations in the cluster state investigated by Wang et al. [1] and consider the steering in this state.

The output modes in terms of the input modes are given by:

$$\begin{aligned}
a_1 &= -\sqrt{(1-R_1)}a_1^{(in)} - \sqrt{R_1}a_2^{(in)} \\
a_2 &= i\sqrt{R_1 R_2}a_1^{(in)} - i\sqrt{(1-R_1)\,R_2}a_2^{(in)} + \sqrt{(1-R_2)}a_3^{(in)} \\
a_3 &= -\sqrt{R_1\,(1-R_2)}a_1^{(in)} + \sqrt{(1-R_1)\,(1-R_2)}a_2^{(in)} - i\sqrt{R_2}a_3^{(in)}
\end{aligned}$$

Hence, the corresponding quadratures for the output modes are:

$$\begin{aligned}
x_1 &= -\sqrt{(1-R_1)}x_1^{(in)} - \sqrt{R_1}x_2^{(in)} \\
x_2 &= -\sqrt{R_1 R_2}p_1^{(in)} + \sqrt{(1-R_1)\,R_2}p_2^{(in)} + \sqrt{(1-R_2)}x_3^{(in)} \\
x_3 &= -\sqrt{R_1\,(1-R_2)}x_1^{(in)} + \sqrt{(1-R_1)\,(1-R_2)}x_2^{(in)} + \sqrt{R_2}p_3^{(in)} \\
p_1 &= -\sqrt{(1-R_1)}p_1^{(in)} - \sqrt{R_1}p_2^{(in)} \\
p_2 &= \sqrt{R_1 R_2}x_1^{(in)} - \sqrt{(1-R_1)\,R_2}x_2^{(in)} + \sqrt{(1-R_2)}p_3^{(in)} \\
p_3 &= -\sqrt{R_1\,(1-R_2)}p_1^{(in)} + \sqrt{(1-R_1)\,(1-R_2)}p_2^{(in)} - \sqrt{R_2}x_3^{(in)}
\end{aligned}$$

where $x_1^{(in)} = e^{-r}x_1^{(0)}$, $x_2^{(in)} = e^{r}x_2^{(0)}$, $x_3^{(in)} = e^{-r}x_3^{(0)}$, $p_1^{(in)} = e^{r}p_1^{(0)}$, $p_2^{(in)} = e^{-r}p_2^{(0)}$ and $p_3^{(in)} = e^{r}p_3^{(0)}$. Here, the superscript 0 denotes the vacuum state.

Using the above expressions, we can calculate the correlations that exist in this state, as given in the work of Wang et al. [1].

$$\begin{aligned}
\Delta^2\left(p_1 - C_{12}x_2\right) &= \left[-\sqrt{(1-R_1)} + C_{12}\sqrt{R_1 R_2}\right]^2 \Delta^2 p_1^{(in)} + \left[\sqrt{R_1} + C_{12}\sqrt{(1-R_1)\,R_2}\right]^2 \Delta^2 p_2^{(in)} \\
&\quad + C_{12}^2\left(1-R_2\right)\Delta^2 x_3^{(in)} \;=\; \frac{(1-R_1)+R_1R_2}{R_1R_2}e^{-2r} \\
\Delta^2\left(p_2 - C_{12}x_1 - C_{23}x_3\right) &= \left[\sqrt{R_1R_2} + C_{12}\sqrt{(1-R_1)} + C_{23}\sqrt{R_1\,(1-R_2)}\right]^2 \Delta^2 x_1^{(in)} \\
&\quad + \left[\sqrt{(1-R_1)\,R_2} - C_{12}\sqrt{R_1} + C_{23}\sqrt{(1-R_1)(1-R_2)}\right]^2 \Delta^2 x_2^{(in)} \\
&\quad + \left[\sqrt{(1-R_2)} - C_{23}\sqrt{R_2}\right]^2 \Delta^2 p_3^{(in)} \;=\; \frac{1}{R_1R_2}e^{-2r} \\
\Delta^2\left(p_3 - C_{23}x_2\right) &= \left[\sqrt{R_1\,(1-R_2)} - C_{23}\sqrt{R_1R_2}\right]^2 \Delta^2 p_1^{(in)} + \left[\sqrt{(1-R_1)\,(1-R_2)} - C_{23}\sqrt{(1-R_1)\,R_2}\right]^2 \Delta^2 p_2^{(in)} \\
&\quad + \left[\sqrt{R_2} + C_{23}\sqrt{(1-R_2)}\right]^2 \Delta^2 x_3^{(in)} \;=\; \frac{1}{R_2}e^{-2r}
\end{aligned}$$

where $C_{12} = \sqrt{(1-R_1)}/\sqrt{R_1R_2}$ and $C_{23} = \sqrt{(1-R_2)}/\sqrt{R_2}$. For $R_1 = 2/3$, these moments have the analytical expressions $\Delta^2\left(p_1 - C_{12}x_2\right) = \frac{1+2R_2}{2R_2}e^{-2r}$, $\Delta^2\left(p_2 - C_{12}x_1 - C_{23}x_3\right) = \frac{3}{2R_2}e^{-2r}$ and $\Delta^2\left(p_3 - C_{23}x_2\right) = \frac{1}{R_2}e^{-2r}$ which are identical to those calculated by Wang et al. and can be found in Eq. (7) in that paper [1].

In the work of Wang et al. [1], a squeezing parameter $r$ is chosen to be 0.345, which corresponds to 3dB squeezing. In the following, we set $R_1 = 2/3$ and study the steering property as a function of $R_2$.

As above, to demonstrate steering for different bipartitions, we consider the quantity $S' = \Delta u' \Delta v' \equiv \Delta\left(h_1 x_1 + g_2 p_2 + h_3 x_3\right) \Delta\left(g_1 p_1 + h_2 x_2 + g_3 p_3\right)$, where

$$\begin{aligned}
\Delta^2 u' &= \Delta^2\left(h_1 x_1 + g_2 p_2 + h_3 x_3\right) \\
&= \left[-h_1\sqrt{1-R_1} + g_2\sqrt{R_1 R_2} - h_3\sqrt{R_1\left(1-R_2\right)}\right]^2 \Delta^2 x_1^{(in)} \\
&\quad + \left[-h_1\sqrt{R_1} - g_2\sqrt{\left(1-R_1\right)R_2} + h_3\sqrt{\left(1-R_1\right)\left(1-R_2\right)}\right]^2 \Delta^2 x_2^{(in)} \\
&\quad + \left(g_2\sqrt{1-R_2} - h_3\sqrt{R_2}\right)^2 \Delta^2 p_3^{(in)}
\end{aligned}$$

and

$$\begin{aligned}
\Delta^2 v' &= \Delta^2\left(g_1 p_1 + h_2 x_2 + g_3 p_3\right) \\
&= \left[g_1\sqrt{1-R_1} + h_2\sqrt{R_1 R_2} + g_3\sqrt{R_1\left(1-R_2\right)}\right]^2 \Delta^2 p_1^{(in)} \\
&\quad + \left[-g_1\sqrt{R_1} + h_2\sqrt{\left(1-R_1\right)R_2} + g_3\sqrt{\left(1-R_1\right)\left(1-R_2\right)}\right]^2 \Delta^2 p_2^{(in)} \\
&\quad + \left(h_2\sqrt{1-R_2} - g_3\sqrt{R_2}\right)^2 \Delta^2 x_3^{(in)}.
\end{aligned}$$

These expressions are used in the steering calculations in the main text Sec. VA4.

## II. THE OBSERVABLES AND GAINS FOR THE CV CLUSTER STATE

For the CV cluster state, in the specific case where $R_1 = 2/3$ and $R_2 = 1/2$, the observables Eqs. (53), (54) and (55) in the main text are given by

$$\begin{aligned}
(S'_{1|23})^2 &= \Delta^2(x_1 - h_{1,2}p_2 + h_{1,3}x_3)\Delta^2(p_1 + g_{1,2}x_2 + g_{1,3}p_3) \\
&= \Big[\frac{1}{3}\left(1 + h_{1,2} + h_{1,3}\right)^2 \Delta^2 x_1^{(in)} + \frac{1}{6}\left(2 - h_{1,2} - h_{1,3}\right)^2 \Delta^2 x_2^{(in)} + \frac{1}{2}\left(h_{1,2} - h_{1,3}\right)^2 \Delta^2 p_3^{(in)}\Big] \\
&\quad \times\Big[\frac{1}{3}\left(1 + g_{1,2} + g_{1,3}\right)^2 \Delta^2 p_1^{(in)} + \frac{1}{6}\left(-2 + g_{1,2} + g_{1,3}\right)^2 \Delta^2 p_2^{(in)} + \frac{1}{2}\left(g_{1,2} - g_{1,3}\right)^2 \Delta^2 x_3^{(in)}\Big]
\end{aligned}$$

$$\begin{aligned}
(S'_{2|13})^2 &= \Delta^2(-p_2 + h_{2,1}x_1 + h_{2,3}x_3)\Delta^2(x_2 + g_{2,1}p_1 + g_{2,3}p_3) \\
&= \Big[\frac{1}{3}\left(h_{2,1} + 1 + h_{2,3}\right)^2 \Delta^2 x_1^{(in)} + \frac{1}{6}\left(2h_{2,1} - 1 - h_{2,3}\right)^2 \Delta^2 x_2^{(in)} + \frac{1}{2}\left(1 - h_{2,3}\right)^2 \Delta^2 p_3^{(in)}\Big] \\
&\quad \times\Big[\frac{1}{3}\left(g_{2,1} + 1 + g_{2,3}\right)^2 \Delta^2 p_1^{(in)} + \frac{1}{6}\left(-2g_{2,1} + 1 + g_{2,3}1\right)^2 \Delta^2 p_2^{(in)} + \frac{1}{2}\left(1 - g_{2,3}\right)^2 \Delta^2 x_3^{(in)}\Big]
\end{aligned}$$

$$\begin{aligned}
(S'_{3|12})^2 &= \Delta^2(x_3 - h_{3,2}p_2 + h_{3,1}x_1)\Delta^2(p_3 + g_{3,2}x_2 + g_{3,1}p_1) \\
&= \Big[\frac{1}{3}\left(h_{3,1} + h_{3,2} + 1\right)^2 \Delta^2 x_1^{(in)} + \frac{1}{6}(2h_{3,1} - h_{3,2} - 1)^2 \Delta^2 x_2^{(in)} + \frac{1}{2}\left(h_{3,2} - 1\right)^2 \Delta^2 p_3^{(in)})\Big] \\
&\quad \times\Big[\frac{1}{3}\left(g_{3,1} + g_{3,2} + 1\right)^2 \Delta^2 p_1^{(in)} + \frac{1}{6}\left(-2g_{3,1} + g_{3,2} + 1\right)^2 \Delta^2 p_2^{(in)} + \frac{1}{2}\left(g_{3,2} - 1\right)^2 \Delta^2 x_3^{(in)}\Big]
\end{aligned}$$

These expressions are used to demonstrate genuine tripartite steering using the criterion in Eq. (56) in the main text.

## III. MONOGAMY CALCULATIONS FOR THE CV SS STATE

We investigate the monogamy inequalities for the CV SS state. We find

$$B_{12} = \frac{1}{4}\left[\Delta^2\left(x_1 - x_2\right) + \Delta^2\left(p_1 + p_2\right)\right] = \frac{5}{8} + \frac{3}{8}e^{-2r}$$
$$B_{13} = \frac{1}{4}\left[\Delta^2\left(x_1 - x_3\right) + \Delta^2\left(p_1 + p_3\right)\right] = \frac{5}{8} + \frac{3}{8}e^{-2r}$$

We note by symmetry of the definition of $B_{ij}$ that $B_{ij} = B_{ji}$. Also, we use

$$S_{1|23}^2 \equiv \Delta^2\left(x_1 - h_2x_2 - h_3x_3\right)\Delta^2\left(p_1 + g_2p_2 + g_3p_3\right)$$
$$= \left[\left(h - \frac{1}{\sqrt{2}}\right)^2 \Delta^2 x_1^{(in)} + \left(h + \frac{1}{\sqrt{2}}\right)\Delta^2 x_2^{(in)}\right]\left[\left(g + \frac{1}{\sqrt{2}}\right)^2 \Delta^2 p_1^{(in)} + \left(g - \frac{1}{\sqrt{2}}\right)^2 \Delta^2 p_2^{(in)}\right]$$

where $h_2 = h_3 = h = \left(\Delta^2 x_1^{(in)} - \Delta^2 x_2^{(in)}\right) / \left[\sqrt{2}\left(\Delta^2 x_2^{(in)} + \Delta^2 x_1^{(in)}\right)\right]$ and $g_2 = g_3 = g = \left(\Delta^2 p_2^{(in)} - \Delta^2 p_1^{(in)}\right) / \left[\sqrt{2}\left(\Delta^2 p_2^{(in)} + \Delta^2 p_1^{(in)}\right)\right]$.

## IV. FOUR-PARTITE STEERING

We now consider four systems, each as a single field mode with boson operator $a_j$ $(j = 1, 2, 3)$. As before, we define the linear combination

$$u = h_1\hat{x}_1 + h_2\hat{x}_2 + h_3\hat{x}_3 + h_4\hat{x}_4$$
$$v = g_1\hat{p}_1 + g_2\hat{p}_2 + g_3\hat{p}_3 + g_4\hat{p}_4 \tag{1}$$

where $h_k$ and $g_k$ $(k = 1, 2, 3,\ 4)$ are real numbers. Using the results of Section II, the following Criterion to detect four-partite steering can be derived. We define numbers $k, l, m, n \in \{1, 2, 3, 4\}$ such that $k \neq l \neq m \neq n$.

***Criterion 1:*** Violation of $\Delta u \Delta v \geq |g_k h_k|$ implies steering of system $k$ by the systems $l$ and $m$ and $n$, and violation of $\Delta u \Delta v \geq |g_l h_l + g_m h_m + g_n h_n|$ implies steering of systems $l$ and $m$ and $n$, by system $k$. Hence, violation of the inequality

$$\Delta u \Delta v \geq \min\Big\{|g_k h_k|, |g_l h_l + g_m h_m + g_n h_n|\Big\} \tag{2}$$

is sufficient to confirm two-way steering across bipartition $k - lmn$. Similarly, violation of $\Delta u \Delta v \geq |g_k h_k + g_l h_l|$ implies steering of $kl$ by $mn$ and violation of $\Delta u \Delta v \geq |g_m h_m + g_n h_n|$ implies steering of $mn$ by $kl$. Hence, violation of the inequality

$$\Delta u \Delta v \geq \min\Big\{|g_k h_k + g_l h_l|, |g_m h_m + g_n h_m|\Big\} \tag{3}$$

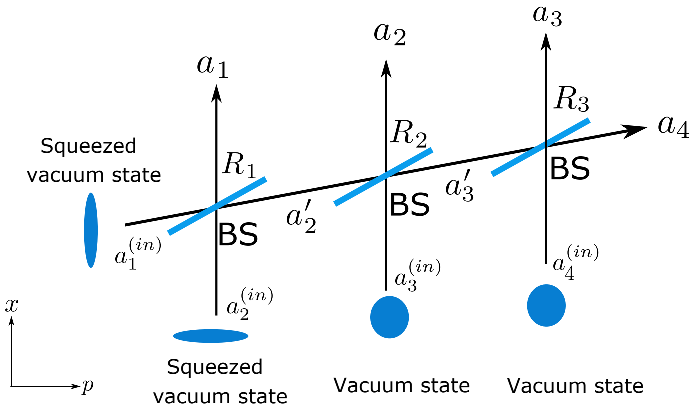


Figure 1. Generation of the 4-partite-entangled CV EPR state. The configuration uses two squeezed-vacuum inputs and two beam splitters (BS) with reflectivities $R_1 = 1/2$, $R_2 = 1/3$, and $R_3 = 1/2$. The $x_i$ and $p_i$ are the two orthogonal quadrature-phase amplitudes of the spatially separated optical modes $i$ $(i = 1, 2, 3, 4)$.

implies two-way steering across bipartition $kl - mn$. The violation of all the conditions for four bipartitions $k - lmn$ $(k = 1, 2, 3, 4)$ and all six conditions for $kl - mn$ implies full 4-partite two-way steering inseparability. If the conditions can be satisfied simultaneously for the same set of $g_i$ and and $h_i$, then one demonstrates genuine four-partite steering. This is a sufficient but not necessary condition. □

Here, we examine the four-partite CV EPR state only (Figures 1 and 2). In particular, we set $h_1 = g_1 = 1$, $h_2 = h_3 = h_4 = h$, and $g_2 = g_3 = g_4 = g$. These values lead to the expressions for $\Delta u \Delta v$ and for the optimal gains $g$ and $h$ given in Section IV. For full 4-partite two-way steering inseparability, the bounds that correspond to different bipartitions in Eq. (2) are $\mathcal{B}_{1|234} = 1$, $\mathcal{B}_{2|134} = \mathcal{B}_{3|124} = \mathcal{B}_{4|123} = |gh|$, $\mathcal{B}_{234|1} = 3\,|gh|$, $\mathcal{B}_{134|2} = \mathcal{B}_{124|3} = \mathcal{B}_{123|4} = |1 + 2gh|$, $\mathcal{B}_{12|34} = \mathcal{B}_{13|24} = \mathcal{B}_{14|23} = |1 + gh|$, and $\mathcal{B}_{23|14} = \mathcal{B}_{24|13} = \mathcal{B}_{34|12} = 2\,|gh|$. Explicitly, the expression for $\Delta u \Delta v$ is given by

$$\Delta u \Delta v = \frac{1}{2}\left\{\left[\left(1+\sqrt{3}h\right)^2 \Delta^2 X_1^{(in)} + \left(1-\sqrt{3}h\right)^2 \Delta^2 X_2^{(in)}\right]\left[\left(1+\sqrt{3}g\right)^2 \Delta^2 P_1^{(in)} + \left(1-\sqrt{3}g\right)^2 \Delta^2 P_2^{(in)}\right]\right\}^{1/2}.$$

The corresponding optimal gains are

$$h = -\frac{\Delta^2 X_1^{(in)} - \Delta^2 X_2^{(in)}}{\sqrt{3}\left[\Delta^2 X_2^{(in)} + \Delta^2 X_1^{(in)}\right]}$$
$$g = -\frac{\Delta^2 P_1^{(in)} - \Delta^2 P_2^{(in)}}{\sqrt{3}\left[\Delta^2 P_2^{(in)} + \Delta^2 P_1^{(in)}\right]}, \qquad (4)$$

where their values for different squeezing parameters $r$ are given in Table I.

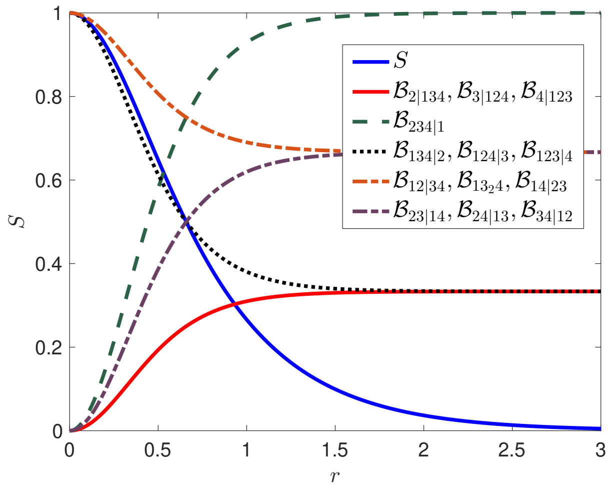


Figure 2. The value of $S = \Delta u \Delta v$ as a function of the squeezing parameter $r$, for a 4-partite CV EPR state. The gains as a function of $r$ are given by the analytical expressions in Section IVA in the main text. The blue solid line corresponds to the value of $S = \mathbf{S}_4$. The remaining lines correspond to the different bounds on the right side of the inequalities Eqs. (2) and (3). When $S$ is smaller than all the bounds, there is genuine 4-partite steering. This is obtained for $r > 0.93$.

| **r** | **4-partite CV EPR** | |
|---|---|---|
| | $h$ | $g$ |
| 0 | 0 | 0 |
| 0.25 | −0.27 | 0.27 |
| 0.50 | −0.44 | 0.44 |
| 0.75 | −0.52 | 0.52 |
| 1.00 | −0.56 | 0.56 |
| 1.50 | −0.57 | 0.57 |
| 2.00 | −0.58 | 0.58 |

Table I. Values of the gains $h$ and $g$ that minimize the variance product in Criterion Eq. (2).

## V. GENERALIZED MONOGAMY RELATION

We provide the proof for the generalized monogamy relation

$$S_{12}S_{13} \geq \frac{\max\left\{1, S_{1|23}\right\}}{\left(1+h_{12}g_{12}\right)\left(1+h_{13}g_{13}\right)} \tag{5}$$

in the main text. Here, $S_{ij} = \Delta\left(x_i - h_{ij}x_j\right)\Delta\left(p_i + g_{ij}p_j\right)/\left(1+h_{ij}g_{ij}\right)$, where $g_{ij}$ and $h_{ij}$ are optimal gains that minimize $S_{ij}$. We note that $S_{ij} < 1$ implies bipartite entanglement [2].

*Proof.* First, recall that $S_{i|j} = \Delta\left(x_i - h_{ij}x_j\right)\Delta\left(p_i + g_{ij}p_j\right)$. Using the inequality $S_{1|2}S_{1|3} \geq 1$ [3]

and dividing this inequality by $(1+h_{12}g_{12})\,(1+h_{13}g_{13})$, we have

$$S_{12}S_{13}=\frac{S_{1|2}S_{1|3}}{(1+h_{12}g_{12})\,(1+h_{13}g_{13})}\geq\frac{1}{(1+h_{12}g_{12})\,(1+h_{13}g_{13})}\,. \tag{6}$$

To show the second part of the inequality, we use the observation that $S_{1|2}\geq S_{1|23}$ and $S_{1|3}\geq S_{1|23}$, which gives

$$S_{12}S_{13}=\frac{S_{1|2}S_{1|3}}{(1+h_{12}g_{12})\,(1+h_{13}g_{13})}\geq\frac{S_{1|23}^{2}}{(1+h_{12}g_{12})\,(1+h_{13}g_{13})}\,. \tag{7}$$

The inequalities Eqs. (6) and (7) lead to the generalized monogamy relation.

---

[1] M. Wang, X. Deng, Z. Qin, and X. Su, Phys. Rev. A **100**, 022328 (2019).
[2] V. Giovannetti, S. Mancini, D. Vitali, and P. Tombesi, Phys. Rev. A **67**, 022320 (2003).
[3] L. Rosales-Zárate, R. Y. Teh, B. Opanchuk, and M. D. Reid, Phys. Rev. A **96**, 022313 (2017).
